# Supplementary material for: SHARP: Short-Window Streaming for Accurate and Robust Prediction in Motion Forecasting
Source: arXiv:2603.28091 source file (2026-03-30)
Supplement: Supplementary file 1 [file _supplementary.tex]

\input{_constants}
\cameraready %

\documentclass[10pt,twocolumn,letterpaper]{article}
\input{cvpr_header}
\myexternaldocument{_main}
\begin{document}

\title{\paperTitle}
\author{\authorBlock}
\maketitlesupplementary

\appendix
\input{_sections/12_appendix}

{\small
\bibliographystyle{ieeenat_fullname}
\bibliography{_sections/_references}
}

\end{document}
